# Supplementary material for: Success Weighted by Completion Time: A Dynamics-Aware Evaluation Criteria for Embodied Navigation
Source: arXiv:2103.08022 source file (2023-10-12)
Supplement: Supplementary file 1 [file old_appendix.tex]

\section{APPENDIX}

\subsection{Hardware setup}
We train each agent on a single computer with 8 GPUs possessing at least 11GB of VRAM, either an RTX 2080Ti or a TITAN V. Training for up to 100M steps across 64 workers in parallel takes approximately 25 hours in wall-clock time.

\subsection{Simulation details}
We use the LoCoBot GLB 3D model from \cite{habitat} to model collisions with the virtual 3D scene invoked by each episode from the Gibson-4+ dataset. In training the three agents presented in this paper, sliding was allowed; in other words, if the robot collided with a wall at a non-perpendicular angle, it would still move along the wall depending on the cosine of the collision angle, rather than coming to a complete stop. 

\subsection{Simultaneous linear and angular control}
The original discrete agent from \cite{ddppo} could only turn or move forward at each time step, but not both. Thus, at each time step, the agent would effectively be instantly translated 0.25m forward or spun 10$^{\circ}$, unless a collision occurred, in which the actual translation would differ as described above. However, for implementing an agent like the continuous action space agent and discrete\_6 that can simultaneously move forward and rotate at the same time, we do not simply translate by the inferred linear displacement and then rotate by the inferred angular displacement (or vice versa). Instead, we leverage Habitat's \cite{habitat} VelocityControl object, which allows us to command the robot to simultaneously assume both a linear and angular velocity, integrating both velocities over time to update the position of the robot. Specifically, we simply set each of these velocities to a value between 0 to 0.25 m/s or -10$^{\circ}$/s to 10$^{\circ}$/s, and then step the simulator physics for 1 second. Unless a collision occurs, this results in the robot taking a curved path during the time step, in which the inferred displacement is manifested as the length of the curved path, rather than the Euclidean distance between its previous and current position.

\subsection{Details about agent alterations}
The architecture and hyperparameters in training the continuous and discrete\_6 agent are identical to the discrete\_4 agent described in \cite{ddppo} except for the differences listed in this subsection and the hardware setup subsection. 

For the continuous agent, as mentioned previously, the final layer outputs parameters for two Gaussian distributions, unlike the final 4-dimensional softmax layer of the discrete\_4 agent. The means and the standard deviations are directly predicted using parallel linear layers that each take inputs from the LSTM policy and output two values, with one layer predicting the means and the other layer predicting the standard deviations. As the standard deviation must be non-negative, it is then bounded to a value between $1\times10^{-6}$ and 1, to limit the amount of stochasticity. After samples are drawn from both parameterized distributions, they are then bounded using a tanh activation function, so that they lie in the interval [-1,1]. These values are then ultimately biased and scaled to map to the 0 to 0.25m and -10$^{\circ}$ to 10$^{\circ}$ ranges. 

For the discrete\_6 agent, to add the new actions we also leverage Habitat's VeloityControl object as mentioned previously, except the forward velocity is fixed at 0.25 m/s for both actions, with one action assuming an angular velocity of -10$^{\circ}$/s and the other assuming 10$^{\circ}$/s. Then, the final layer is changed from a 4-dimensional softmax to a 6-dimensional softmax that parameterizes a categorical distribution to sample from.
